# Supplementary material for: In Defence of Visual Analytics Systems: Replies to Critics
Source: arXiv:2201.09772 source file (2022-08-06)
Supplement: Supplementary file 1 [file app1Section.tex]

\section{Comparison between our eight-component framework with others}
We compare our eight-component framework in~\autoref{fig:sections} with existing ones to inform our readers.
As shown in~\autoref{fig:section_compare},
our framework is an integrated adaption of the nine-stage design study framework for information visualization~\cite{sedlmair2012design} and the visual analytics model by Keim~\ea~\cite{keim2008visual}.
The rough mapping is not intended to provide a template or precise guidelines on how to write a VA system manuscript,
but rather for helping our readers, especially for those who are unfamiliar with VA systems, understand our definition and scope for each component in our framework.

\textbf{Compared with the nine-stage design study framework.}
The first three stages (\ie~learn, winnow, and cast) are collectively called as the precondition phase which focuses on ``preparing the visualization researcher for the work, and finding and filtering synergistic collaborations with domain experts''~\cite{sedlmair2012design}.
They are in general prior to the actual research progress and thus researchers tend not to detail them in the writing.

The core phrase including four stages (\ie~discover, design, implement, and deploy) is the core of a design study.
The discover stage concerns with domain experts to characterize and abstract problem, which is mapped to our problem abstraction component.
The design stage involves designing an information visualization solution.
However,
in the context of visual analytics,
it involves designing not only the visualization but also the data processing (data mining) methods~\cite{keim2008visual}.
The implement stage concerns implementing the system software prototype.
Finally,
the deploy stage requires ``deploying a tool and gathering feedback about its use in the wild''~\cite{sedlmair2012design},
which maps to the Evaluation component.

The last phrase consists of reflecting and writing.
We map reflecting to discussion and conclusion,
and map writing to all components in our framework.

\textbf{Compared with the visual analytics model.}
The VA model by Keim~\ea~\cite{keim2008visual} consists of four components, namely data, model (automated data analysis), visualization (visual data exploration), and knowledge.
The merge the data and model into a single Data and Processing component,
which is a common practice in our surveyed paper (\autoref{table:secHeading}).
The visualization is mapped to Visual Design,
whereas knowledge is linked to Evaluation since it is common to report analysis insights in case studies or usage scenarios.

\begin{figure}[!t]
	\centering
	\includegraphics[width=1\linewidth]{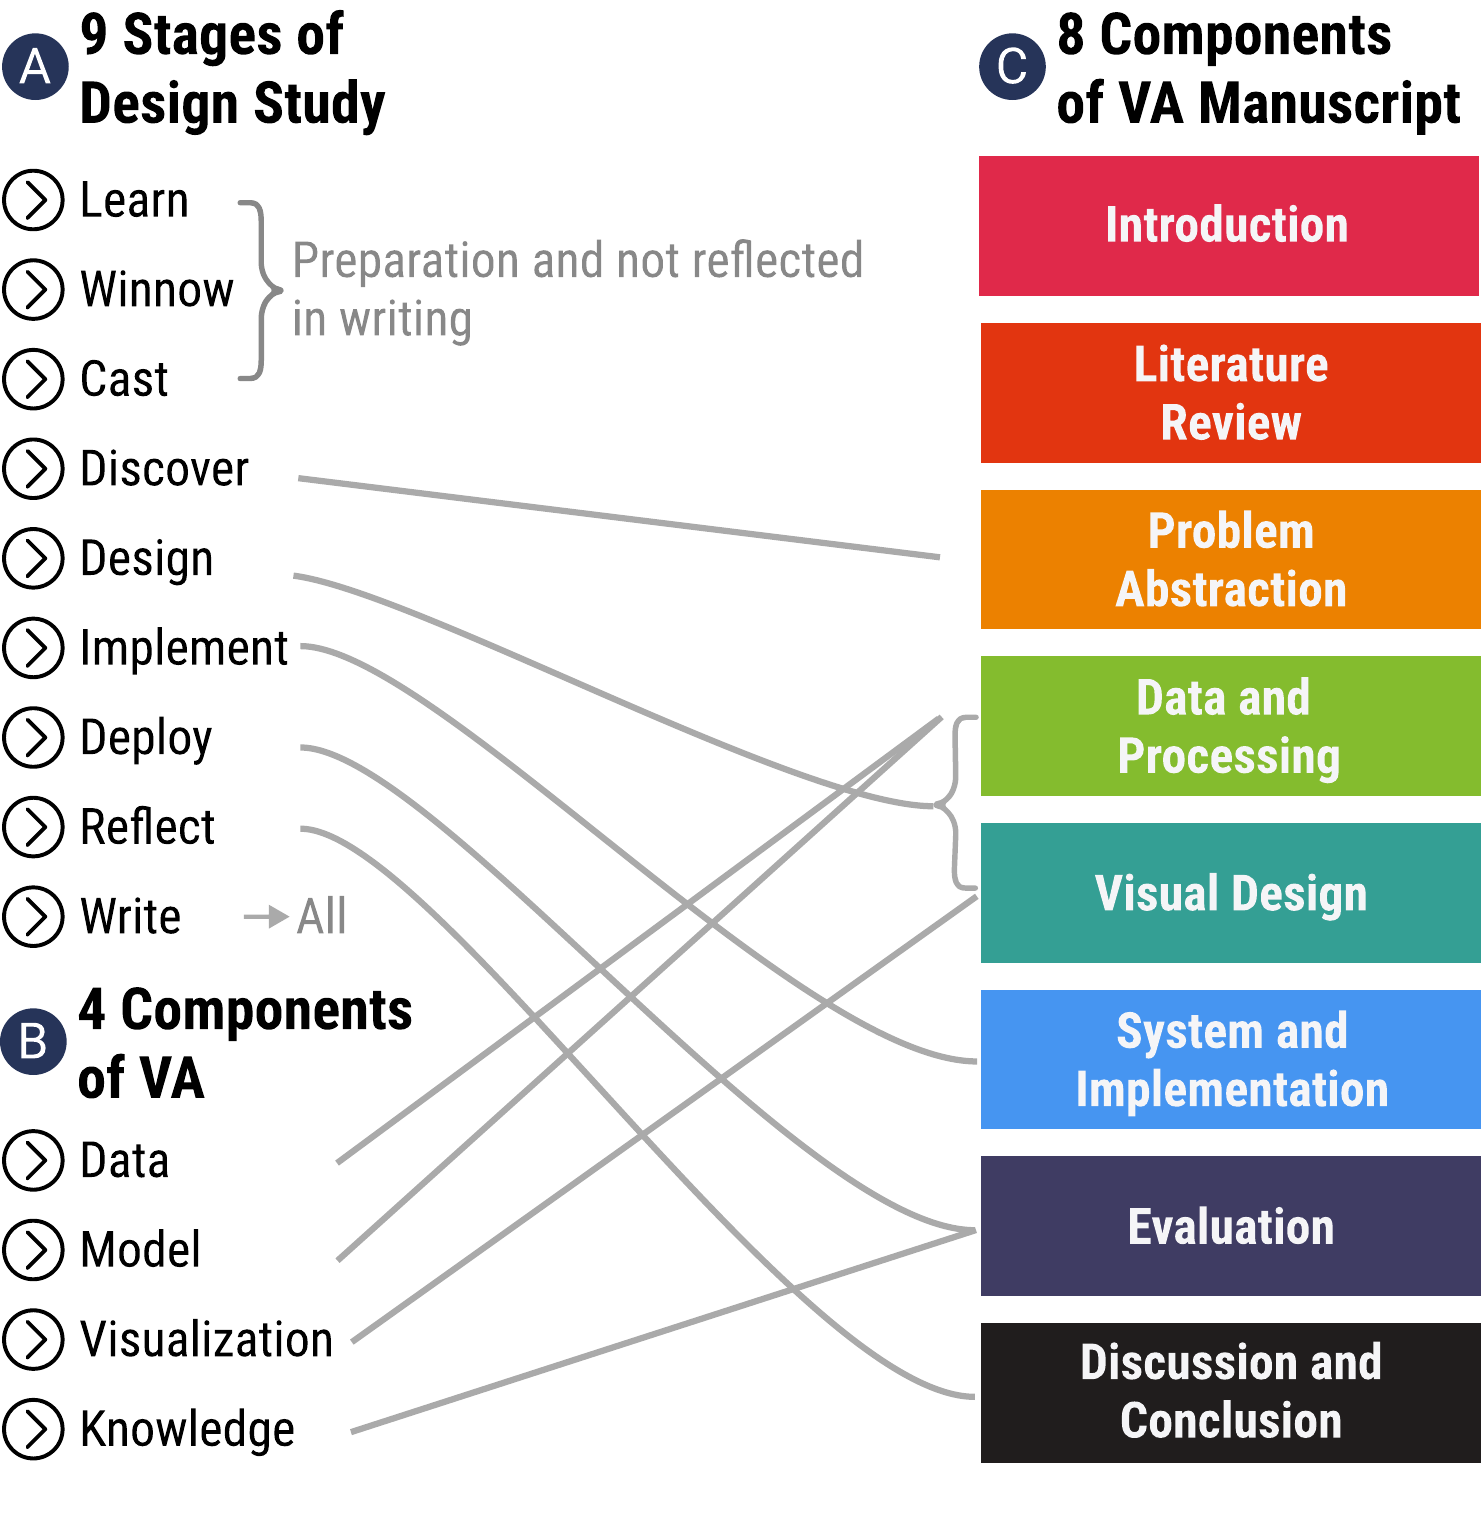}
	\caption{Relationships of our eight-component framework to the nine-stage framework of design study~\cite{sedlmair2012design} and the visual analytics framework~\cite{keim2008visual}.}
	\label{fig:section_compare}
\end{figure}

\section{Alternative Approaches to Group Criticisms}
We considered three methods for grouping the criticisms and finally decided the aforementioned eight-component framework.
In the following text, 
we discuss each alternative and explain our design choices.

\textbf{Rejected}: grouping by review guidelines. Our first attempt was to refer to criteria in review guidelines. Lee~\ea~\cite{lee2019beyond} in the IEEE VIS 2018 Tutorial \textit{Beyond Paper Types: How to Evaluate and Communicate VIS Research Contributions} listed seven issues including originality, technical soundness, relevance, claims, evaluation, writing, and overall quality. However, we found them to be high-level and not specific to our scope. For instance, we had internal disagreement about ``insufficient justifications of visual designs'' fell into technical soundness, claims, or writing.

\textbf{Rejected}: grouping by visualization design frameworks. We next referred to existing visualization design frameworks including Munzner's nested model~\cite{munzner2009nested},
nine-stage framework of design studies~\cite{sedlmair2012design}, and their extensions~\cite{syeda2020design, sedlmair2016design}.
However, their discussions primarily focus on information visualization systems instead of visual analytics systems,
\eg the design stage in the nine-stage framework is defined as ``the generation and validation of data abstractions, visual encodings, and interaction mechanisms''~\cite{sedlmair2012design}.
However,
VA systems often involve advance data mining algorithms that are separately designed, implemented, and evaluated~\cite{chen2019ontological}.

\textbf{Accepted}: grouping by manuscript components. Our final decision was to group criticisms by their corresponding components or sections in the manuscript. This was reasonable since it is expected that the writing should in general conform to the design progress and outcomes~\cite{sedlmair2012design}. We also found it feasible to identify common components from exiting research manuscripts (\autoref{fig:sections}). We emphasized that we by no means intended to propose a template that might stifle innovated ideas,
but instead to use such common patterns to guide our analysis and discussion.
