# Supplementary material for: In Defence of Visual Analytics Systems: Replies to Critics
Source: arXiv:2201.09772 source file (2022-08-06)
Supplement: Supplementary file 2 [file app2VIS2021.tex]

\begin{table*}[]
\small
\caption{Mappings between our eight-component framework to section headings in 31 surveyed papers in IEEE VIS 2021}
\label{table:secHeading}
\centering
\begin{tabular}{l|p{14cm}}
\toprule
\textbf{Ours} & \textbf{Section Headings} \\ \hline
Introduction & Introduction [31] \\
Related Work & Related work [29], Background [2], Working with hyperproperties [1], Background on bitcoin mining and mining pools [1], Background and related work [1] \\
Problem Abstraction & Background [7], Design goals [2], Design requirements [2], Methods [1], Design of coux [1], Analytic tasks [1], Task and design requirements [1], Design process and task analysis [1], Analysis factors and motivation [1], Risk-aware framework [1], Design challenges [1], Human-ai teaming for zero-shot classification [1], Tasks and workflow [1], Domain-centered design [1], Abstractions [1], Formative study [1], Informing the design [1], Design overview [1], Collaboration and domain goals [1], Biological background [1], Design methodology [1], Background and design requirements [1], User-centered design [1], Domain background [1], Development process and requirement analysis [1] \\
Data and Algorithms & Algorithm [2], Non-visual data analysis support [1], Dataset description [1], Predictive modeling [1], Data analysis [1], Data and analysis [1], Scalable neural network summarizationneurocartography [1], Data acquisition [1], Efficient dynamic clustering [1], A multilevel overview of event sequences [1], Vision based autonomous driving models [1], Geo-context aware data processing [1], Method [1], Model [1] \\
Visual Design & Visual design [3], Visualization design [2], Loon visualization design [1], Visualization and interaction [1], Vbridge [1], User interface [1], Visualization techniques [1], Design of the visualization system [1] \\
System and Implementation & Implementation [4], Overview [2], System design [2], The irvine system [1], M2 lens [1], Visual evaluation approach [1], Lumos [1], Design of visqa [1], Evis [1], Visualization system [1], Architecture [1], Visualization techniques [1], Semantic navigator [1], System implementation [1], System description [1], Coux system [1], System overview [1], Vitality [1], Visual analytics framework [1], Hypervis [1], Visual analysis of disease progression [1], Visual analytics system [1] \\
Evaluation & Evaluation [13], Case studies [4], Usage scenarios [3], User study [2], Expert evaluation [2], User evaluation [2], Example usage scenarios [2], Usage scenarios and expert review [1], Validating hypervis [1], Results [1], Experimental validation [1], Evaluation and results [1], Human experiment to evaluate neurocartography [1], Usage scenario [1], Experiments [1], Expert feedback [1], Motivating case study [1], Evaluation with domain experts [1], Use cases [1], System evaluation [1], Case study [1], Case studies and evaluation [1] \\
Discussion and Conclusion & Discussion [21], Conclusion [15], Conclusion and future work [3], Discussion and conclusion [3], Limitations [2], Discussions [2], Lessons learned and reflections [1], Conclusions [1] \\
\bottomrule
\end{tabular}
% \begin{tablenotes}
%   \small
%   \item **: D and V refer to the top-level sections that cover both Data and Algorithms (D) and Visual Design (V). 
% \end{tablenotes}
\end{table*}

\section{Analysis of Research Papers in IEEE VIS 2021}
We perform literature review on research papers published at IEEE VIS 2021 to inform some of our decisions such as the naming of eight components in VA system manuscript (\autoref{fig:sections}).
In this section,
we describe our corpus and analysis results.

\subsection{Corpus}
To keep our corpus manageable and necessarily representative,
we decided to survey research papers in IEEE VIS 2021,
which was both recent and premium.
Three authors of this work held a meeting to scan all research instances and decided whether each instance fell into our scope.
Out of the 111 instances,
we finally found 30 research papers (27\%), 
which was a considerably large portion.
The sample size was also comparable to that in Lam~\ea~\cite{lam2017bridging}'s research where 20 design study papers published in IEEE InfoVis were analyzed to ``bridge from goals to tasks''.
In the following text, 
we provide several typical excluded papers to help readers understand our scope.

% \begin{compactitem}
%     \item We excluded research that did not claim itself to be ``visual analytics system'', \eg~COVID-view~\cite{jadhav2021covid}.
%     \item We excluded research that did not target at a specific domain problem, \eg~SightBi~\cite{}
% \end{compactitem}

\subsection{Sections' Naming}
We analyze the top-level section headings of those research papers and mapp them to our eight components.
Not surprisingly we find complex mapping relationships as shown in~\autoref{table:secHeading}.
We observe a general one-to-one or one-to-many mapping for three components, \ie~\textit{Introduction}, \textit{Related Work}, and \textit{Discussion and Conclusion},
which are mostly generic in academic papers.
We identify most variations for \textit{Problem Abstraction},
and thus decide our wording that we consider to informative and self-descriptive.
We find many-to-many mappings for \textit{Data and Algorithms} and \textit{Visual Design},
for instance,
many research papers merged them into a single \textit{System and Implementation} section.
For this reason,
we only map system-level and implemented issues to~\textit{System and Implementation} in our list of criticisms (\autoref{table:pitfal}).
Finally,
for \textit{Evaluation},
we find different evaluation methods that resulted into different names such as case studies and usage scenarios.

In summary,
our analysis result suggests that the writing styles are diverse, changing, and innovative.
We present our eight-component framework as one feasible way of organizing writing,
which benefits our discussions.
We encourage readers to take our framework as a starting point for creating, discussing, and validating alternative ideas.

\subsection{Contribution Types}
We code and analyze the contribution types as claimed by the authors in surveyed literature.
As shown in~\autoref{table:contributions},
we identify 11 types of contribution types.
The most frequent claimed contribution is the evaluation (28),
followed by VA systems/tools/prototypes (24) and open-sourced VA systems/tools/prototypes (3).
In addition to implemented systems or tools,
a large number of research claims the design, workflow, or the framework of visual analytics as contributions (19).

From the design study perspective,
nine research instances claim the design study and problem abstraction as a contribution.
Besides,
two papers discuss new application domains that not previously appeared in the visualization literature.
From the technique perspective,
some surveyed papers contribute novel visual representation (10) and data mining algorithms (8).
Finally, 
we find other contribution types that are relatively rare,
including reflection (2), data model (1), and dataset (1).

In conclusion,
our surveyed research mainly contributes evaluation, VA frameworks, systems, problem abstraction, novel visual representation and data mining algorithms,
which conforms to our eight-component framework.
This suggests that evaluating VA system research requires an overall consideration over those components.
However, we note that reflections tend not to appear common,
despite ongoing calls for the use of reflection to generate general knowledge from applied visualization research~\cite{meyer2018reflection}.
